# Supplementary material for: LiFF: Light Field Features in Scale and Depth
Source: arXiv:1901.03916 ancillary file (2019-01-13)
Supplement: Supplementary file 1 [file LiFF_Supplemental.pdf]

# Supplementary Material

## LiFF: Light Field Features in Scale and Depth

Donald G. Dansereau<sup>1,2</sup>, Bernd Girod<sup>1</sup>, and Gordon Wetzstein<sup>1</sup>

<sup>1</sup>Stanford University, <sup>2</sup>The University of Sydney

### I. THE MULTI-VIEW LIGHT FIELD DATASET

The multi-view light field (LF) dataset is, to our knowledge, the first large dataset of its kind. All images were captured with a hand-held Lytro Illum camera, and each scene photographed from a diversity of camera poses. The individual LFs have small baselines, on the order of a centimeter, while the camera poses vary over a broader baseline, on the order of a meter or more. This emulates the case of a single, mobile lenslet-based LF camera, or multiple LF cameras operating simultaneously.

The dataset contains 4211 LFs organized into 30 categories. There are 850 scenes, with most scenes captured from between 4 and 6 poses. There are examples of scenes with as few as 3 poses, and some with 7 or more. A set of ‘clusters’ files identify which images belong in each scene. The dataset is available at <http://lightfields.stanford.edu/mvlf>.

#### A. Camera

The dataset was collected with a single hand-held Lytro Illum camera. Focus, zoom, and exposure settings were not fixed, but vary from image to image. Metadata and calibration data for the camera, including flat-field images, are included with the dataset.

#### B. Light Fields

The file formats included in the dataset are depicted in Fig. 1. Each image is available as a raw Lytro LFR file and a decoded ESLF file, with LFRs and ESLFs available as separate downloads. Decoding either file type requires the calibration data from the camera, which is available with the dataset.

LFR files contain the raw lenslet image as stored on the camera. They have  $7728 \times 5368$  pixels, 12 bits of Bayer-coded colour depth, and about  $14 \times 14$  pixels per lenslet in a hexagonal grid that is not pixel-aligned. These can be decoded using an open-source toolbox [4] or the Lytro Power Tools. Each LFR occupies about 55 MBytes of space.

ESLF files are a decoded LF format that has been de-Bayered and pixel-aligned to an orthogonal grid of lenslet images. These are easy to load and interpret as a 2D array of 2D images, i.e. a 4D LF. The ESLF files in the dataset were produced using the Lytro Power Tools Beta, and stored as PNG files with  $7574 \times 5250$  pixels. There are  $14 \times 14$  pixels per lenslet and about  $541 \times 375$  lenslets, though this varies between LFs. In addition to de-Bayering and aligning, the Lytro tool also applies rectification, reducing the appearance of lens distortion. We applied lossless PNG compression and

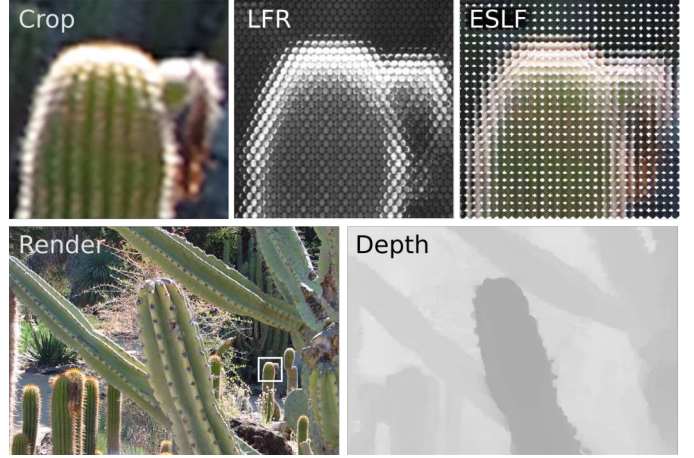

Fig. 1. File types included in the dataset: (bottom) a 2D render and depth map as produced by the Lytro Power Tools, and (top) a crop of the 2D render, a raw LFR file, and a de-Bayered, aligned, and rectified ESLF file. Also included is a per-LF metadata file specifying camera settings including zoom, focus, exposure, and gain settings.

reduced the bit depth to 8 bits per channel yielding an average file size of 50 MBytes.

Each LF is accompanied by a metadata file, rendered extended-depth-of-field 2D image, and a depth map, also generated using the Lytro Power Tools. The metadata file includes focus, zoom, exposure, and gain settings. The rendering settings for producing the extended-depth-of-field images are included in the dataset.

#### C. Depth Maps

A point in 3D space appears in the LF as a plane with slope inversely proportional to the point’s depth [1], [3], [5]. The depth values produced by the Lytro Power Tools describe the image created inside the camera by the main lens. These can be related to the slope as it appears in the sampled LF with enough information about the microlens and pixel geometry. It can also be related to the 3D shape of the scene with enough information about the main lens. Note that the depth maps are estimates, they are not ground truth nor are they a gold standard for depth estimation from LFs [6].

Each pixel of the depth map encodes a ratio  $\lambda$ , with the mapping from grayscale provided in a separate metadata file. Referring to Fig. 2,  $\lambda$  is the distance of a point’s image inside the camera to the microlens array, divided by the focal length of the microlenses:

$$\lambda = \frac{d_I}{d_\mu}. \quad (1)$$

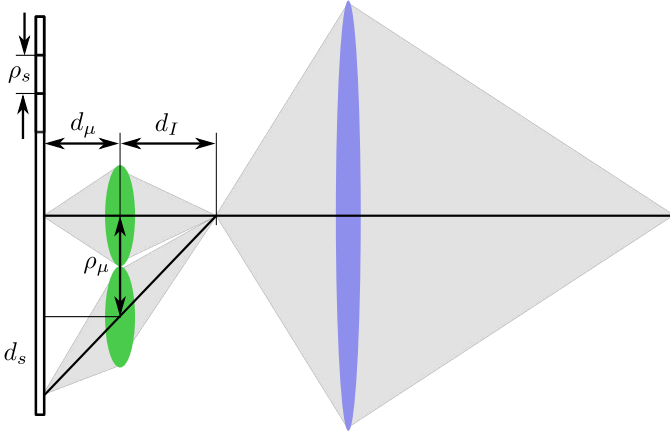

Fig. 2. Geometry relating  $\lambda$  from the depth map files to slope observed in the sampled LF – see Sect. I-C. A scene point (right) imaged through the main lens (blue) forms an image inside the camera. This in turn is imaged by the microlenses (green) onto the sensor (left).

For images behind the microlenses,  $d_I$  and  $\lambda$  are negative.  $\lambda$  can be related to the slopes appearing in the sampled LFs following the similar triangles in the figure,

$$\frac{d_s}{d_\mu} = \frac{\rho_\mu}{d_I}, \quad (2)$$

where  $\rho_\mu$  is the lenslet pitch, and  $d_s$  is the the apparent motion of a point when moving from one lenslet to the next, i.e. the continuous-domain slope. It is convenient to use the inverse of this slope, and to convert to pixels for the sampled LF:

$$m = \frac{\rho_s}{d_s}, \quad (3)$$

where  $\rho_s$  is the pixel pitch. Combining the above we find

$$m = \frac{\rho_s}{\rho_\mu} \lambda. \quad (4)$$

For the Illum,  $\rho_s = 1.4\mu\text{m}$ ,  $\rho_\mu = 20\mu\text{m}$ , and  $d_\mu = 40\mu\text{m}$ , so

$$m = \frac{1.4}{20} \lambda. \quad (5)$$

A point at the focal plane of the camera will be focused on the microlens array, and have  $\lambda = 0$ ,  $m = 0$ . This makes sense since we know a point at the camera’s focal plane appears only beneath a single microlens. Objects beyond the focal plane will appear with positive  $\lambda$  and slope, while objects closer than the focal plane will have negative  $\lambda$  and slope, as expected. Manual inspection shows that the slopes appearing in the dataset’s ESLF-encoded LFs agree well with the  $\lambda$  values in the depth maps following (5).

Relating slopes to depths in the scene is also possible. The main metadata file specifies  $\lambda_\infty$ , the  $\lambda$  corresponding to an object at infinity, as well as the effective focal length of the main lens, for the particular camera zoom and focus settings used to take each photo. This is enough information to transform  $\lambda$  to depth via the thin lens equation, though the accuracy of estimates resulting from this approach is unclear. Depth estimation from LFs is an active area of research [2], [4], [6], [7].

Most LFs in the dataset contain substantial depth variation, see for example Figs. 1 and 3. A histogram of the occurrence

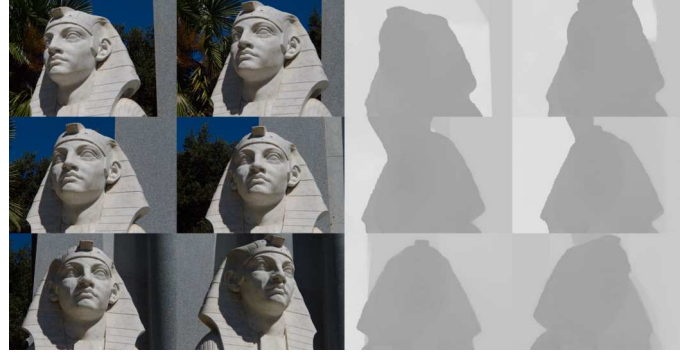

Fig. 3. Six views of a scene shown alongside the Lytro-generated depth maps.

of slopes over all pixels of all images in the dataset, based on the  $\lambda$  values in the depth maps, is shown in Fig. 4. Most scene content falls between slopes of  $\pm 1$ .

#### D. Scenes

Scenes fall into one of 30 categories, listed in Table I along with the numbers of scenes and images appearing in each category. The distribution of image counts per scene is shown in Table II.

Scenes are of typical indoor office and outdoor urban campus environments. They include Lambertian and non-Lambertian surfaces, fine and coarse occlusion, specularity, transparency, translucency, and subsurface scattering. No particular attempt was made to emphasize challenging content. Examples of the types of images contained in the dataset are shown in Fig. 5, and example multi-view sequences are shown in Fig. 6.

There is moderate motion blur in some of the scenes, caused by motion / shake of the hand-held camera. This is especially true for indoor scenes where illumination was lower, though there are also some outdoor scenes with motion blur. Some scenes contain dynamic elements, e.g. moving people and swaying vegetation, and this content will not be consistent between camera poses. An effort was made to keep dynamic content to a minimum.

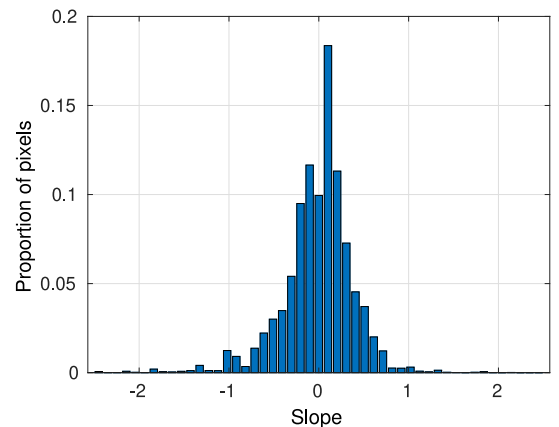

Fig. 4. Histogram of slopes appearing in the dataset, based on the depth maps; most content appears between  $\pm 1$ .

| Image category | Scene count | Image count |
|----------------|-------------|-------------|
| Bamboo         | 10          | 49          |
| Batteries      | 5           | 28          |
| Benches        | 21          | 97          |
| Bikes          | 18          | 83          |
| Books          | 5           | 27          |
| Bottles        | 7           | 37          |
| Boxes          | 30          | 177         |
| Buildings      | 66          | 283         |
| Cables         | 40          | 230         |
| Cacti          | 16          | 83          |
| Chairs         | 3           | 14          |
| Coins          | 7           | 33          |
| Cups           | 15          | 80          |
| Drawers        | 2           | 9           |
| Fire Hydrants  | 3           | 12          |
| Flowers        | 189         | 872         |
| Glasses        | 8           | 40          |
| Glue           | 5           | 30          |
| Keyboards      | 9           | 44          |
| Leaves         | 141         | 719         |
| Misc           | 30          | 167         |
| Pens & Pencils | 26          | 136         |
| Phones         | 5           | 27          |
| Screws         | 9           | 47          |
| Shelf          | 5           | 23          |
| Signs          | 38          | 186         |
| Succulents     | 19          | 94          |
| Tables         | 23          | 115         |
| Tools          | 12          | 70          |
| Trees          | 83          | 399         |
| Total          | 850         | 4211        |

TABLE I

THE 30 CATEGORIES PRESENT IN THE DATASET, ALONG WITH THE SCENE COUNT AND IMAGE COUNT FOR EACH CATEGORY.

| Images per scene | Count |
|------------------|-------|
| 3                | 27    |
| 4                | 250   |
| 5                | 343   |
| 6                | 197   |
| 7                | 29    |
| 9                | 1     |
| 10               | 1     |
| 13               | 1     |

TABLE II

OCCURRENCE OF IMAGE COUNTS PER SCENE: ALL SCENES HAVE AT LEAST 3 IMAGES, MOST HAVE BETWEEN 4 AND 6, AND A FEW HAVE 7 OR MORE.

## REFERENCES

- [1] E. H. Adelson and J. Y. A. Wang. Single lens stereo with a plenoptic camera. *IEEE Transactions on Pattern Analysis and Machine Intelligence (TPAMI)*, 14(2):99–106, 1992.
- [2] Y. Bok, H.-G. Jeon, and I. S. Kweon. Geometric calibration of micro-lens-based light-field cameras using line features. In *Computer Vision–ECCV 2014*, pages 47–61. Springer, 2014.
- [3] R. Bolles, H. Baker, and D. Marimont. Epipolar-plane image analysis: An approach to determining structure from motion. *Intl. Journal of Computer Vision (IJCV)*, 1(1):7–55, 1987.
- [4] D. G. Dansereau, O. Pizarro, and S. B. Williams. Decoding, calibration and rectification for lenselet-based plenoptic cameras. In *Computer Vision and Pattern Recognition (CVPR)*, pages 1027–1034. IEEE, June 2013.
- [5] I. Ihrke, J. Restrepo, and L. Mignard-Debise. Principles of light field imaging. *IEEE Signal Processing Magazine*, 1053(5888/16), 2016.
- [6] O. Johannsen, K. Honauer, B. Goldluecke, A. Alperovich, F. Battisti, Y. Bok, M. Brizzi, M. Carli, G. Choe, M. Diebold, et al. A taxonomy and evaluation of dense light field depth estimation algorithms. In *Computer Vision and Pattern Recognition (CVPR) Workshops*, pages 1795–1812, 2017.
- [7] Y. Xu, K. Maeno, H. Magahara, and R. I. Taniguchi. Camera array calibration for light field acquisition. *Frontiers of Computer Science*, 9(5):691–702, 2015.

## E. Conclusion

It is our hope that this dataset will enable a broad range of research into multi-view LF processing including registration, calibration, structure-from-motion, interpolation, and feature extraction.

**Acknowledgments** This work was supported in part by the NSF/Intel Partnership on Visual and Experiential Computing (Intel #1539120, NSF #IIS-1539120).

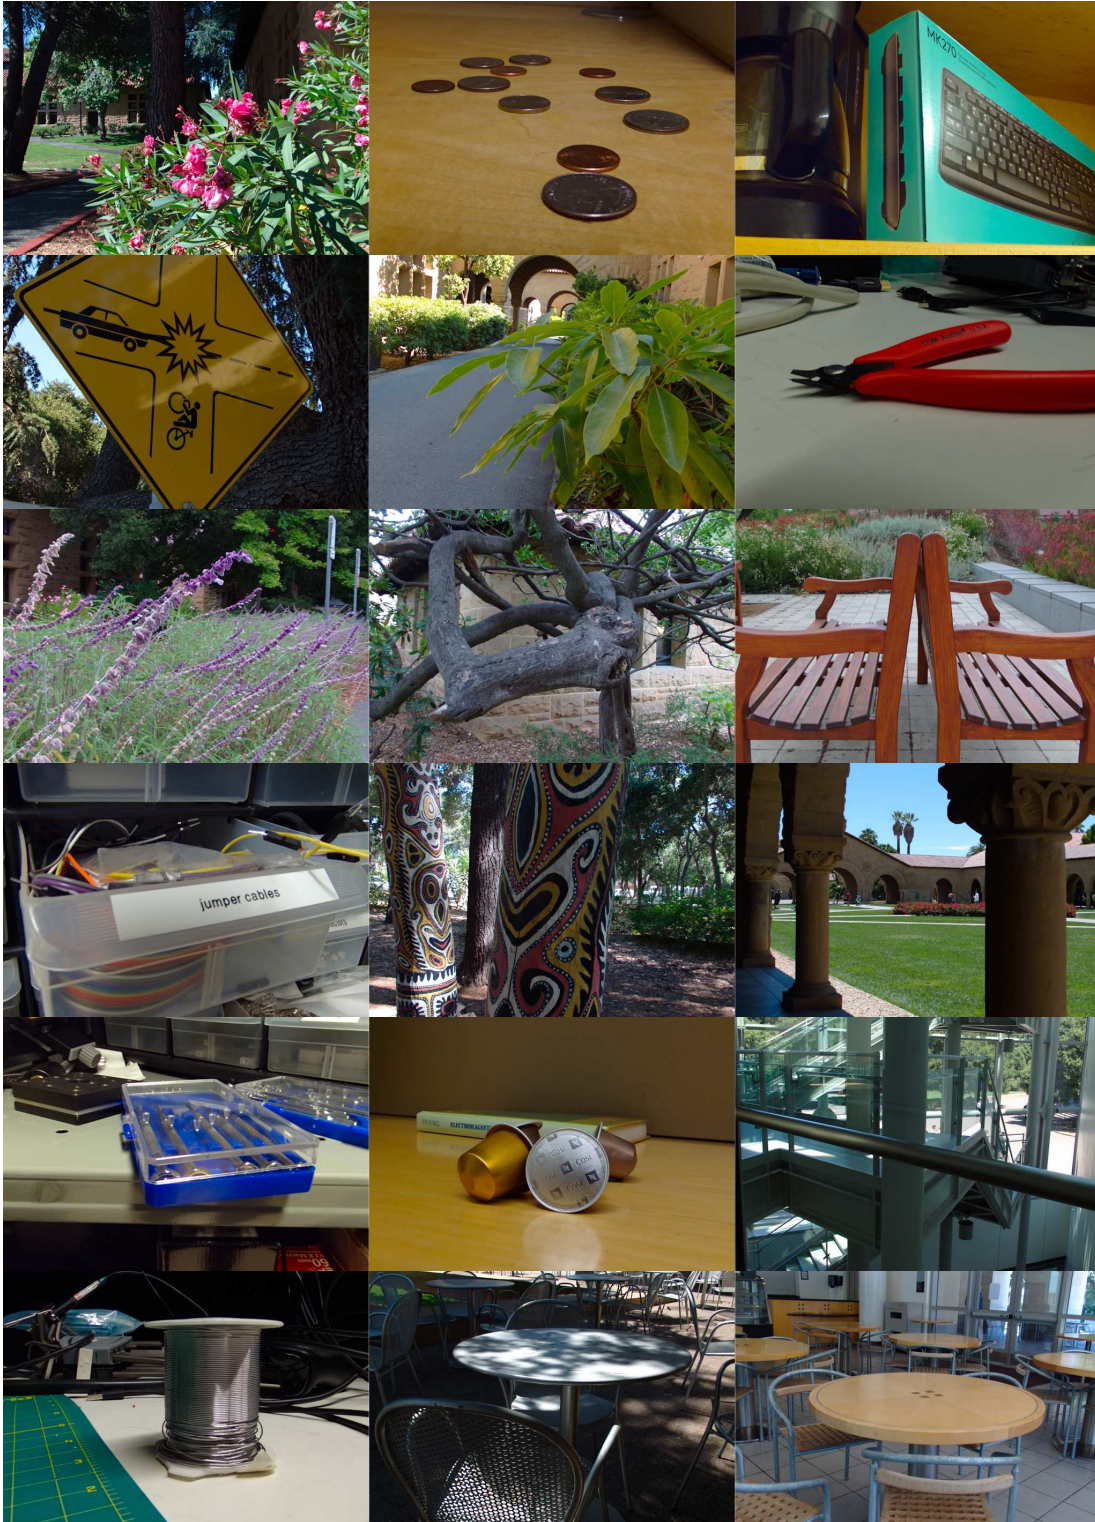

Fig. 5. A collection of 2D renders showing typical scene content contained in the dataset.

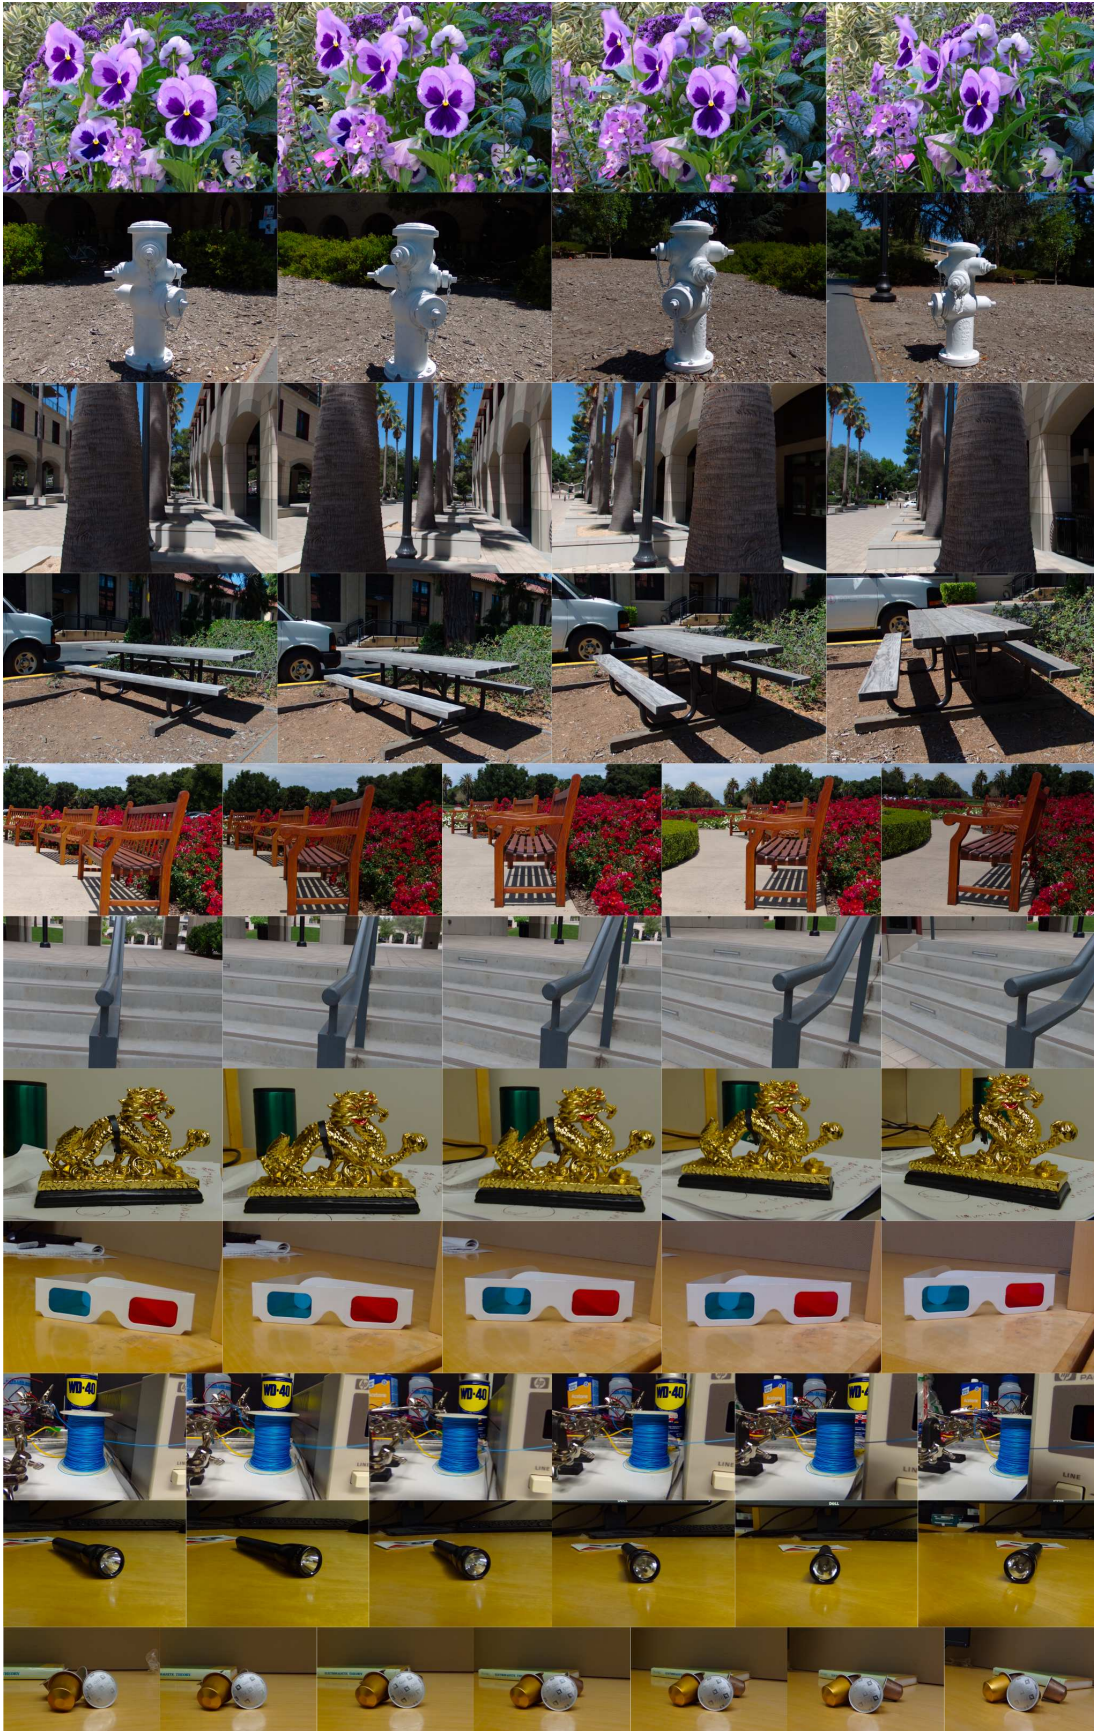

Fig. 6. A set of multi-pose sequences of between 4 and 7 images showing the typical view diversity of the dataset.
